# Supplementary material for: Microscopic Derivation of Ginzburg-Landau Theory and the BCS Critical Temperature Shift in General External Fields
Source: arXiv:2210.09356 source file (2023-02-11)
Supplement: Supplementary file 1 [file 10_Appendix_A.tex]

%auto-ignore  % for ArXiv to process correctly

\section{The Eigenvalues of the Periodic Landau Hamiltonian}
\label{Spectrum_Landau_Hamiltonian_Section}

In this appendix, we investigate the eigenvalues of the periodic Landau Hamiltonian and their multiplicity. We shall fix an arbitrary charge $q\in \Nbb$ and we consider the space $\Lmag^{q,2}(Q_B)$ of $L^2_{\mathrm{loc}}(\Rbb^3)$-functions $\Psi$, which are gauge-perodic with respect to the magnetic translations
\begin{align}
T_{B,q}(v)\Psi(x) &:= \e^{\i \frac{q\Bbold}{2}\cdot (v \wedge x)} \Psi(x+v), & v &\in \Rbb^3, \label{Magnetic_Translation_charge-q}
\end{align}
of the lattice $\Lambda_B$ defined above \eqref{Fundamental_cell}, that is, these functions satisfy $T_{B, q}(\lambda)\Psi = \Psi$ for every $\lambda\in \Lambda_B$. The magnetic translations obey $T_{B,q}(v+w) = \e^{\i \frac{q\Bbold}{2} \cdot (v\wedge w)} T_{B, q}(v) T_{B,q}(w)$, whence the group $\{T_{B,q}(\lambda)\}_{\lambda\in \Lambda_B}$ is abelian.

On the Sobolev space $\Hmag^{q,2}(Q_B)$ of gauge-periodic functions, where
\begin{align}
\Hmag^{q,m}(Q_B) &:= \bigl\{ \Psi\in \Lmag^{q,2}(Q_B) :  \Pi^\nu \Psi\in \Lmag^{q, 2} (Q_B) \quad \forall \nu\in \Nbb_0^3, |\nu|_1\leq m\bigr\} \label{Periodic_Sobolev_Space_charge-q}
\end{align}
for $m\in \Nbb_0$, we consider the Landau Hamiltonian $\Pi_q^2$ with magnetic momentum given by $\Pi_q :=-\i \nabla + q \Abold$. This operator commutes with the translations in \eqref{Magnetic_Translation_charge-q} and the magnetic flux through the unit cell $Q_B$ is equal to $2\pi q$, see \eqref{Fundamental_cell} and the discussion below \eqref{Fundamental_cell}. In this respect, Sections \ref{Magnetically_Periodic_Samples} and \ref{Periodic Spaces} correspond to the special cases $q=1$ and $q=2$, respectively.

%Since $\Pi_q^{(3)}$ commutes with $\Pi_q^{(1)}$ and $\Pi_q^{(2)}$, we will be able to diagonalize $(\Pi_q^{(3)})^2$ independently of $(\Pi_q^{(1)})^2 + (\Pi_q^{(2)})^2$. As it turns out, the eigenvalues of the latter operator are not even sensitive to 
%In particular, this holds if $\lambda\in \Lambda_B$ is an integer multiple of $b_3$, where $b_i = \sqrt{2\pi B^{-1}} \, e_i$ are the basis vectors spanning $\Lambda_B$. 
We choose a Bloch--Floquet decomposition $\Ucal_{\mathrm{BF}}$ (see also Section \ref{Schatten_Classes}) such that $\Pi_q$ fibers according to
\begin{align}
\Ucal_{\mathrm{BF}} \, \Pi_q \, \Ucal_{\mathrm{BF}}^* =  \int_{[0,1)^3}^\oplus \dd \vartheta \; \Pi_q(\vartheta) \label{Bloch-Floquet-decomposition}
\end{align}
with fiber momentum operators
\begin{align*}
\Pi_q(\vartheta) := -\i \nabla + q\Abold + \sqrt{2\pi B} \, \vartheta
\end{align*}
acting on the magnetic Sobolev space $\Hmag^{q,2}(Q_B)$ in \eqref{Periodic_Sobolev_Space_charge-q}.
%on the box $Q_B$ with periodic boundary conditions.
%\begin{align*}
%\Hcal_{\mathrm{mag}}^{q,2}(Q_B) := \Bigl\{ \Psi\in L^2(Q_B) : (-\i\nabla + q\Abold)^\nu \Psi\in L^2(Q_B) \quad \forall \nu\in \Nbb_0^3, |\nu|_1\leq m ; \; \e^{\i \frac{q\Bbold}{2} \cdot (b_i \wedge x) T_{B,q}(b_i)(\lambda)}\Psi(0) = \Psi(0) \bigr\}
%\end{align*}

\begin{prop}
\label{Spectrum_Landau_Hamiltonian}
For every $B >0$, $q\in \Nbb$, and $\vartheta\in [0, 1)^3$, the spectrum of $\Pi_q(\vartheta)^2$ consists of the isolated eigenvalues
\begin{align}
E_{q,B, \vartheta}(k, p) &:= q \, B \, (2k+1) + 2\pi \, B \, (p + \vartheta_3)^2, & k\in \Nbb_0, \; p\in \Zbb. \label{Spectrum_Landau_Hamiltonian_eq1}
\end{align}
Furthermore, their multiplicity is finite and equals
\begin{align}
\dim \ker ( \Pi_q(\vartheta)^2 - E_{q,B, \vartheta}(k, p)) = q.
%\begin{cases} 2q & p^2>0,\\ q & p^2 =0.\end{cases} 
\label{Spectrum_Landau_Hamiltonian_eq2}
\end{align}
\end{prop}

In preparation for the proof, we first note that,  by rescaling, $\Pi_q(\vartheta)^2$ is isospectral to $B \, (-\i \nabla + \frac q2 e_3\wedge x+ \sqrt{2\pi}\, \vartheta )^2$. We henceforth assume that $B =1$.

Furthermore, we introduce the notation $x = (x_\perp , x_3)^t$ and define the two-dimensional operator $\Pi_{\perp, q}(\vartheta) := (\Pi_q^{(1)}(\vartheta), \Pi_q^{(2)}(\vartheta))^t$. This operator acts on functions $\psi_\perp$ satisfying the gauge-periodic condition $T_{\perp,q} (\lambda) \psi_\perp = \psi_\perp$ for all $\lambda \in \sqrt{2\pi}\, \Zbb^2$ with
\begin{align}
T_{\perp,q} (v) \psi_\perp(x) &:= \e^{\i \frac{q}{2} (v_1x_2 - v_2x_1)}  \psi_\perp(x + v),  & v &\in \Rbb^2.
\end{align}

The following result is well known, even for more general lattices, see for example \cite[Proposition 6.1]{Tim_Abrikosov}. We include the proof for the sake of completeness, adding the treatment of the perturbation by $\vartheta$.

\begin{lem}
\label{Spectrum_Landau_Hamiltonian_Lemma}
For every $q\in \Nbb$, the spectrum of the operator $\Pi_{\perp, q}(\vartheta)^2$ consists of the isolated eigenvalues $E_q(k) := (2k+1)q$, $k\in \Nbb_0$. Each of $E_q(k)$ is $q$-fold degenerate.
\end{lem}

\begin{proof}
Since $[\Pi_q^{(1)}(\vartheta), \Pi_q^{(2)}(\vartheta)] = -\i q$, the creation and annihilation operators
\begin{align}
a(\vartheta) &:= \frac{1}{\sqrt{2q}} \bigl( \Pi_q^{(1)}(\vartheta) - \i \Pi_q^{(2)}(\vartheta)\bigr), & a^*(\vartheta) &:= \frac{1}{\sqrt{2q}} \bigl( \Pi_q^{(1)}(\vartheta) + \i \Pi_q^{(2)}(\vartheta)\bigr) \label{Creation-Annihilation}
\end{align}
satisfy $[a(\vartheta), a^*(\vartheta)] = 1$ and it is easy to show that
\begin{align}
\Pi_q(\vartheta)^2 = q\, (2\,  a^*(\vartheta) a(\vartheta) + 1). \label{Spectrum_Landau_Hamiltonian_eq3}
\end{align}
From this, we read off the formula for $E_q(k)$.

The rest of the proof is devoted to the statement about the degeneracy. First, with the help of the creation and annihilation operators, it is easy to show that the degeneracy of $E_q(k)$ is equal to that of $E_q(0)$ for all $k\in \Nbb_0$. Therefore, it is sufficient to determine the degeneracy of $E_q(0)$. By \eqref{Spectrum_Landau_Hamiltonian_eq3},  $\ker(\Pi_{\perp, q}^2(\vartheta) - q)$ equals $\ker(a(\vartheta))$ so it suffices to determine the latter. A straightforward calculation shows that
\begin{align*}
\e^{\frac q4 |x_\perp - \frac 2q \sqrt{2\pi} J\vartheta|^2} \; a(\vartheta) \; \e^{-\frac q4|x_\perp - \frac 2q \sqrt{2\pi} J\vartheta|^2} &= - \frac{\i}{\sqrt{2q}} \, [  \partial_{x_1} - \i \partial_{x_2}], & J := \bigl(\begin{matrix} & -1 \\ 1\end{matrix}\bigr).
\end{align*}
Therefore, the property $\psi_\perp \in\ker a(\vartheta)$ is equivalent to the function $\xi := \e^{\frac q4 |x_\perp - \frac 2q \sqrt{2\pi} J\vartheta|^2} \psi_\perp$ satisfying $\partial_{x_1}\xi - \i \partial_{x_2}\xi =0$. If we identify $z = x_1 + \i x_2\in \Cbb$, then $J\vartheta = \i (\vartheta_1 + \i \vartheta_2)$ and this immediately implies that the complex conjugate function $\ov \xi$ solves the Cauchy-Riemann differential equations, whence it is entire. We define the entire function
\begin{align*}
\Theta(z) := \e^{-2\i z \Re \vartheta} \, \e^{-\frac{q}{2\pi} (z - \frac{2\pi \i}{q}   \vartheta)^2} \; \ov {\xi \Bigl( \sqrt{\frac 2\pi} \, z\Bigr)}. %= \e^{-2\i z \Re \vartheta} \e^{\frac{q}{2\pi} (|z - \i \frac{2\pi}{q} \vartheta|^2 - (z - \frac{2\pi}{q}\i  \vartheta)^2)} \; \ov{ \psi_\perp \Bigl( \sqrt{\frac 2\pi} \, z\Bigr)}.
\end{align*}
A tedious calculation shows that the gauge-periodicity of $\psi_\perp$ is equivalent to the relations
\begin{align}
\Theta(z + \pi) &= \Theta(z), \label{Spectrum_Landau_1}\\ 
\Theta(z + \i \pi) &= \e^{-2\pi \vartheta} \, \e^{-2\i q z}\,  \e^{q\pi} \,  \Theta(z). \label{Spectrum_Landau_2}
\end{align}
Therefore, it suffices to show that the space of entire functions $\Theta$ which obey \eqref{Spectrum_Landau_1} and \eqref{Spectrum_Landau_2} is a vector space of dimension $q$. We claim that \eqref{Spectrum_Landau_1} implies that $\Theta$ has an absolutely convergent Fourier series expansion of the form
\begin{align}
\Theta(z) = \sum_{k\in \Zbb} c_k \; \e^{2\i kz}. \label{Spectrum_Landau_3}
\end{align}
To prove this, we first note that, for fixed imaginary part $x_2$, we may expand $\Theta$ in an absolutely convergent series $\Theta(z) = \sum_{k\in \Zbb} a_k(x_2) \e^{2\i kx_1}$ with
\begin{align*}
a_k(x_2) = \frac 1\pi \int_0^\pi \dd x_1 \; \e^{-2\i k x_1} \, \Theta(x_1 + \i x_2).
\end{align*}
By the Cauchy-Riemann equations, it is easy to verify that $a_k' = -2k\, a_k$. Therefore, the number $c_k := \e^{2k x_2} \, a_k(x_2)$ is independent of $x_2$ and provides the expansion \eqref{Spectrum_Landau_3}. Furthermore, \eqref{Spectrum_Landau_2} implies that $c_{k+q} = \e^{-\pi (2k+q)} \e^{2\pi \vartheta} c_k$. Therefore, the series \eqref{Spectrum_Landau_3} is fully determined by the values of $c_0, \ldots, c_{q-1}$ and we conclude that1³³1³³1³³1111 $\ker a(\vartheta)$ is a $q$-dimensional vector space.
\end{proof}

\begin{proof}[Proof of Proposition \ref{Spectrum_Landau_Hamiltonian}]
As mentioned before, it suffices to prove the proposition for $B = 1$. It is easy to verify that for any $\vartheta \in [0,1)^3$ the spectrum of $(\Pi_q(\vartheta)^{(3)})^2$ consists of the simple eigenvalues $2\pi\, (p+ \vartheta_3)^2$ with $p\in \Zbb$. Since $\Pi_q(\vartheta)^{(3)}$ and $\Pi_{\perp,q}(\vartheta)$ commute, Lemma \ref{Spectrum_Landau_Hamiltonian_Lemma} implies the existence of an orthonormal basis of eigenvectors for $\Pi_q(\vartheta)^2$ of the form $\psi_\perp^{k, m}(x_\perp) \psi_3^{\vartheta, p}(x_3)$ with $k\in \Nbb_0$, $m = 1, \ldots, q$ and $p\in \Zbb$, corresponding to the eigenvalue $E_{q,1, \vartheta}(k,p)$. This proves the formulas \eqref{Spectrum_Landau_Hamiltonian_eq1} and  \eqref{Spectrum_Landau_Hamiltonian_eq2}.
\end{proof}
