# Supplementary material for: Microscopic Derivation of Ginzburg-Landau Theory and the BCS Critical Temperature Shift in General External Fields
Source: arXiv:2210.09356 source file (2023-02-11)
Supplement: Supplementary file 2 [file 11_Appendix_B.tex]

%auto-ignore  % for ArXiv to process correctly
